# Supplementary material for: Fast, Precise Myelin Water Quantification using DESS MRI and Kernel Learning
Source: arXiv:1809.08908 source file (2018-09-24)
Supplement: Supplementary file 1 [file supp.tex]

% reset counters
\setcounter{section}{0}
\setcounter{equation}{0}
\setcounter{figure}{0}
\setcounter{table}{0}
\setcounter{page}{1}
\makeatletter

% supplement headers

% supplement equations

% supplement floats
